# Supplementary material for: Disentangling Structured Components: Towards Adaptive, Interpretable and Scalable Time Series Forecasting
Source: arXiv:2305.13036 source file (2024-02-15)
Supplement: Supplementary file 1 [file Appendix.tex]

\section{Appendix}

\begin{figure*}[thb]
\centering
\subfloat[PeMSD7.]{
\includegraphics[width=0.8\linewidth]{figure/pems_sample.pdf}
}

\subfloat[Electricity.]{
\includegraphics[width=0.8\linewidth]{figure/elec_sample.pdf}
\label{fig:elec_sample}
}

\subfloat[BikeNYC.]{
\includegraphics[width=0.8\linewidth]{figure/bike_sample.pdf}
}
\caption{For each of (a), (b) and (c), the left figure shows the probability density function of the observed values aggregated from all variables at all time steps, and the right figure displays some sample time series.}
\label{fig:data_dist}
\end{figure*}
